# Supplementary material for: HexTiles and Semantic Icons for MAUP-Aware Multivariate Geospatial Visualizations
Source: arXiv:2407.16897 source file (2026-11-06)
Supplement: Supplementary file 1 [file supplementary.tex]

\subsection{Another use case for HexTiles on wildfire detection data in California's Central Valley}

sd
